# Supplementary material for: Crowdsourcing Impacts: Exploring the Utility of Crowds for Anticipating Societal Impacts of Algorithmic Decision Making
Source: arXiv:2207.09525 source file (2022-07-19)
Supplement: Supplementary file 1 [file appendix.tex]

\begin{appendix}

\section{Appendix}

\end{appendix}
